# Supplementary material for: Enhanced diffusivity in microscopically reversible active matter
Source: arXiv:2102.11821 ancillary file (2022-08-25)
Supplement: Supplementary file 1 [file suppl_enhanced_diffusivity.pdf]

# SUPPLEMENTAL MATERIAL
# Enhanced diffusivity of microscopically reversible active matter


Artem Ryabov*

*Charles University, Faculty of Mathematics and Physics,*
*Department of Macromolecular Physics, V Holešovičkách 2, 180 00 Praha 8, Czech Republic*
*Departamento de Física, Faculdade de Ciências, Universidade de Lisboa, 1749-016 Lisboa, Portugal and*
*Centro de Física Teórica e Computacional, Faculdade de Ciências,*
*Universidade de Lisboa, 1749-016 Lisboa, Portugal*

Mykola Tasinkevych†

*Departamento de Física, Faculdade de Ciências, Universidade de Lisboa, 1749-016 Lisboa, Portugal*
*Centro de Física Teórica e Computacional, Faculdade de Ciências,*
*Universidade de Lisboa, 1749-016 Lisboa, Portugal and*
*SOFT Group, School of Science and Technology,*
*Nottingham Trent University, Clifton Lane, Nottingham NG11 8NS, UK*


This Supplemental Material consists of three sections providing mathematical derivations of the results discussed in the main. First, in Sec. I, we solve the master equation describing thermodynamically consistent active dynamics in a constant external field and provide explicit formulas for the first two moments of the particle position. In Sec. II, by performing a continuum limit we obtain thermodynamically consistent coarsegrained Langevin equations. Similar limiting procedures have been discussed recently e.g. in Refs. [1–3]. The derivation presented in Sec. II of this Supplemental Material is similar in spirit to the one from Ref. [2]. In addition to what is discussed in Ref. [2], we incorporate into the derivation an external force and show how to renormalize the active velocity such that a comparison with the phenomenological ABP (Active Brownian Particle) model becomes straightforward. In Sec. III, we derive first two moments of the particle position based on the thermodynamically consistent coarsegrained Langevin equation derived in Sec. II.

## I. POSITION STATISTICS FOR ACTIVE JUMP-DIFFUSION PROCESS

Particle's orientation is described by the unit vector $\boldsymbol{n}(t)$ having components $\boldsymbol{n}(t) = (\cos\phi(t), \sin\phi(t))$. It undergoes rotational Brownian motion with the diffusion coefficient $D_{\rm r}$. Hence the angle $\phi(t)$ between directions of $\boldsymbol{n}(t)$ and the $x$ axis, satisfies the Langevin equation

$$\frac{d\phi}{dt} = \sqrt{2D_{\rm r}}\,\xi_{\rm r}(t), \tag{S1}$$

where the Gaussian white noise $\xi_{\rm r}(t)$ obeys $\langle \xi_{\rm r}(t)\rangle = 0$ and $\langle \xi_{\rm r}(t)\xi_{\rm r}(t')\rangle = \delta(t-t')$. Integration of this Langevin equation yields

$$\phi(t) = \phi_0 + \sqrt{2D_{\rm r}}\int_0^t dt'\,\xi_{\rm r}(t'). \tag{S2}$$

In all following calculations, the initial value $\phi(0) = \phi_0$ is assumed to be a random variable homogeneously distributed over the interval $[0, 2\pi)$.

Position of the particle center of mass, $\boldsymbol{r}(t)$, is a functional of the process $\phi(t)$. For any given trajectory of $\phi(t)$, generated in accordance with Eq. (S2), we can describe $\boldsymbol{r}(t)$ by the probability density function (PDF) $P(\boldsymbol{r}, t)$. In case of the active motion in a constant force field discussed in the main text, it satisfies the master equation

$$\partial_t P(\boldsymbol{r},t) = k_+(t)P(\boldsymbol{r}-\boldsymbol{n}(t)\delta r,t) + k_-(t)P(\boldsymbol{r}+\boldsymbol{n}(t)\delta r,t) - [k_+(t)+k_-(t)]\,P(\boldsymbol{r},t) - \mu\boldsymbol{\nabla}\cdot[\boldsymbol{F}P(\boldsymbol{r},t)] + D\boldsymbol{\nabla}^2 P(\boldsymbol{r},t), \tag{S3}$$

where the last two terms correspond to passive diffusion of the particle. Since $\boldsymbol{n}(t)$ in this equation is a stochastic function of time, the moments of $\boldsymbol{r}(t)$ calculated based on $P(\boldsymbol{r},t)$ should be also averaged over all realizations of the process $\phi(t)$.

---


* artem.ryabov@mff.cuni.cz
† mtasinkevych@fc.ul.pt

In Subsec. I A we give general results for $\langle \boldsymbol{r}(t)\rangle$ and $\langle \boldsymbol{r}^2(t)\rangle$, which are independent of a particular form of rates $k_\pm(t)$. Further, in Subsec. I B, we assume the activated rates from the main text, where $k_\pm(t)$ depend exponentially on $\delta W(t)$, $\delta W(t) = -F\delta r\cos\phi(t)$, and evaluate general results of Subsec. I A for this specific scenario. Subsec. I C gives particle moments and effective diffusion coefficient in the limit $F\delta r/2k_\mathrm{B}T < 1$ and Subsec. I D summarizes all formulas for $F = 0$.

### A. General results for time-dependent rates $k_\pm(t)$

To derive moments of the particle position $\boldsymbol{r}(t)$, we introduce the moment generating function $\varphi(\boldsymbol{k},t)$, $\boldsymbol{k} = (k_x, k_y)$, defined as

$$\varphi(\boldsymbol{k},t) = \int d\boldsymbol{r} P(\boldsymbol{r},t)\,\mathrm{e}^{\boldsymbol{k}\cdot\boldsymbol{r}}. \tag{S4}$$

In accordance with (S3), it satisfies the first-order linear differential equation

$$\partial_t\varphi(\boldsymbol{k},t) = L(\boldsymbol{k},t)\varphi(\boldsymbol{k},t), \tag{S5}$$

where

$$L(\boldsymbol{k},t) = k_+(t)\left[\mathrm{e}^{\boldsymbol{k}\cdot\boldsymbol{n}(t)\delta r} - 1\right] + k_-(t)\left[\mathrm{e}^{-\boldsymbol{k}\cdot\boldsymbol{n}(t)\delta r} - 1\right] + \mu(\boldsymbol{k}\cdot\boldsymbol{F}) + D(\boldsymbol{k}\cdot\boldsymbol{k}). \tag{S6}$$

Solution of Eq. (S5) subject to the initial condition $\varphi(\boldsymbol{k},0) = 1$ [initially, the particle position is $\boldsymbol{r}(0) = 0$] is

$$\varphi(\boldsymbol{k},t) = \exp\left[\int_0^t dt' L(\boldsymbol{k},t')\right]. \tag{S7}$$

We calculate the first two moments of coordinates $x(t)$ and $y(t)$ based on partial derivatives of $\varphi(\boldsymbol{k},t)$ with respect to components of the vector $\boldsymbol{k} = (k_x, k_y)$. The derivatives are evaluated at $\boldsymbol{k} = \boldsymbol{0}$ and averaged over all realizations of the process $\phi(t)$:

$$\langle x(t)\rangle = \left\langle \int_0^t dt'\partial_{k_x} L(\boldsymbol{0},t')\right\rangle, \tag{S8}$$

$$\langle y(t)\rangle = \left\langle \int_0^t dt'\partial_{k_y} L(\boldsymbol{0},t')\right\rangle, \tag{S9}$$

$$\langle x^2(t)\rangle = \left\langle \int_0^t dt'\partial^2_{k_xk_x} L(\boldsymbol{0},t') + \left[\int_0^t dt_1\partial_{k_x} L(\boldsymbol{0},t_1)\right]^2\right\rangle, \tag{S10}$$

$$\langle y^2(t)\rangle = \left\langle \int_0^t dt'\partial^2_{k_yk_y} L(\boldsymbol{0},t') + \left[\int_0^t dt_1\partial_{k_y} L(\boldsymbol{0},t_1)\right]^2\right\rangle. \tag{S11}$$

Equations (S8) and (S9) yield following expressions for the mean values of $x(t)$ and $y(t)$

$$\langle x(t)\rangle = \mu F t + \delta r\int_0^t dt'\langle[k_+(t') - k_-(t')]\cos\phi(t')\rangle, \tag{S12}$$

$$\langle y(t)\rangle = \delta r\int_0^t dt'\langle[k_+(t') - k_-(t')]\sin\phi(t')\rangle, \tag{S13}$$

respectively. Furthermore, because $\phi_0$ is random, i.e., its values are homogeneously distributed in $[0, 2\pi)$, we have $\langle y(t)\rangle = 0$ regardless of a specific form of $k_\pm(t)$. For this we need to assume that the rates depend on the particle orientation through $\delta W(t)$ only. Then $[k_+(t') - k_-(t')]$ is a function of $\cos\phi(t')$ and can be formally expanded into a power series in powers of $[\cos\phi(t')]$. Each term of such series will vanish after it is multiplied by $\sin\phi(t')$ and averaged with respect to $\phi_0$ over the interval $[0, 2\pi)$ due to the orthogonality of sin and cos functions.

Expressions for second moments of $x(t)$ and $y(t)$ are algebraically more involved. To present them in a compact form, we introduce the notation

$$\Delta k(t) = k_+(t) - k_-(t). \tag{S14}$$

Then the second central moments, calculated based on the formulas (S8)-(S11) are given by

$$\langle x^2(t)\rangle - \langle x(t)\rangle^2 = 2Dt + (\delta r)^2 \int_0^t dt' \langle [k_+(t') + k_-(t')] \cos^2 \phi(t')\rangle + \\ + (\delta r)^2 \int_0^t dt_1 \int_0^t dt_2 \, [\langle \Delta k(t_1) \cos\phi(t_1) \Delta k(t_2) \cos\phi(t_2)\rangle - \langle \Delta k(t_1)\cos\phi(t_1)\rangle\langle \Delta k(t_2)\cos\phi(t_2)\rangle] \,, \tag{S15}$$

$$\langle y^2(t)\rangle - \langle y(t)\rangle^2 = 2Dt + (\delta r)^2 \int_0^t dt' \langle [k_+(t') + k_-(t')] \sin^2 \phi(t')\rangle + \\ + (\delta r)^2 \int_0^t dt_1 \int_0^t dt_2 \langle \Delta k(t_1) \sin\phi(t_1) \Delta k(t_2) \sin\phi(t_2)\rangle. \tag{S16}$$

Summing these equations, we get the variance of the particle position at time $t$:

$$\langle \boldsymbol{r}^2(t)\rangle - \langle \boldsymbol{r}(t)\rangle^2 = 4Dt + (\delta r)^2 \int_0^t dt' \langle [k_+(t') + k_-(t')]\rangle + (\delta r)^2 \int_0^t dt_1 \int_0^t dt_2 \langle \Delta k(t_1)\Delta k(t_2) \cos[\phi(t_2) - \phi(t_1)]\rangle \\ - (\delta r)^2 \int_0^t dt_1 \int_0^t dt_2 \langle \Delta k(t_1)\cos\phi(t_1)\rangle\langle \Delta k(t_2)\cos\phi(t_2)\rangle. \tag{S17}$$

### B. Results for activated rates and arbitrary $k_\pm^{(0)}$

Let us factorize $k_\pm(t)$ as products of rates $k_\pm^{(0)}$ describing a force-free active propulsion and of the force-dependent part as

$$k_\pm(t) = k_\pm^{(0)} \exp\left[\pm \frac{F\delta r \cos\phi(t)}{2k_{\mathrm{B}}T}\right]. \tag{S18}$$

Then Correlation functions under the integrals in Eqs. (S12) and (S17) then can be evaluated recalling an integral representation of the modified Bessel functions of the first kind [4]:

$$\int_0^{2\pi} \frac{d\phi}{2\pi} \cos(n\phi) \exp[z\cos(\phi)] = \mathrm{I}_n(z), \tag{S19}$$

where $n$ is an integer, $z$ is a real number, and $\mathrm{I}_n(.)$ denotes the modified Bessel function of the first kind of order $n$ [4].

Using Eq. (S19) and the antisymmetry $\mathrm{I}_1(-z) = -\mathrm{I}_1(z)$, we get

$$\langle k_\pm(t)\cos\phi(t)\rangle = \pm k_\pm^{(0)} \, \mathrm{I}_1\left(\frac{F\delta r}{2k_{\mathrm{B}}T}\right), \tag{S20}$$

which yields the explicit results for the mean coordinate $x(t)$. It reads

$$\langle x(t)\rangle = \left[\mu F + \delta r (k_+^{(0)} + k_-^{(0)}) \, \mathrm{I}_1\left(\frac{F\delta r}{2k_{\mathrm{B}}T}\right)\right] t. \tag{S21}$$

Let us now evaluate all terms in on the right-hand side of Eq. (S17). The mean value under the integral over $t'$ follows from the formula (S19):

$$\langle [k_+(t') + k_-(t')]\rangle = (k_+^{(0)} + k_-^{(0)}) \, \mathrm{I}_0\left(\frac{F\delta r}{2k_{\mathrm{B}}T}\right). \tag{S22}$$

Mean values $\langle \Delta k(t_j)\cos\phi(t_j)\rangle$, $j = 1, 2$ follow from Eq. (S20), we get

$$\langle \Delta k(t_1)\cos\phi(t_1)\rangle\langle \cos \Delta k(t_2)\phi(t_2)\rangle = (k_+^{(0)} + k_-^{(0)})^2 \, \mathrm{I}_1^2\left(\frac{F\delta r}{2k_{\mathrm{B}}T}\right). \tag{S23}$$

Explicit evaluation of the correlation function $\langle \Delta k(t_1)\Delta k(t_2)\cos[\phi(t_2)-\phi(t_1)]\rangle$ will be performed first assuming $t_2 > t_1 \geq 0$. Then we decompose the process $\phi(t)$ into its initial value and increments:

$$\phi(t_1) = \phi_1 + \phi_0, \tag{S24}$$
$$\phi(t_2) = \phi_2 + \phi_1 + \phi_0, \tag{S25}$$

where $\phi_1 = \sqrt{2D_{\rm r}}\int_0^{t_1} dt'\xi_{\rm r}(t')$, and $\phi_2 = \phi(t_2)-\phi(t_1) = \sqrt{2D_{\rm r}}\int_{t_1}^{t_2} dt'\xi_{\rm r}(t')$. Accordingly, increments $\phi_j$, $j=1,2$, are independent zero-mean Gaussian random variables with variances $2D_{\rm r}\Delta t_j$, where $\Delta t_1 = t_1$, and $\Delta t_2 = t_2 - t_1$. The probability density function for the increment $\phi_j$ is given by

$$p(\phi_j) = \frac{1}{\sqrt{4\pi D_{\rm r}\Delta t_j}}\exp\left(-\frac{\phi_j^2}{4D_{\rm r}\Delta t_j}\right), \qquad j = 1,2. \tag{S26}$$

Furthermore, the initial value $\phi_0$ is homogeneously distributed in the interval $[0, 2\pi)$.

The difference $\Delta k(t_j)$, Eq. (S14), depends on $\phi(t_j)$. To make this dependence explicit, we introduce the auxiliary function $\kappa$ defined as

$$\kappa(\phi_1+\phi_0) = \Delta k(t_1), \tag{S27}$$
$$\kappa(\phi_2+\phi_1+\phi_0) = \Delta k(t_2). \tag{S28}$$

The correlation function $\langle \Delta k(t_1)\Delta k(t_2)\cos[\phi(t_2)-\phi(t_1)]\rangle$ then is written as

$$\langle \Delta k(t_1)\Delta k(t_2)\cos[\phi(t_2)-\phi(t_1)]\rangle = \int_{-\infty}^{+\infty} d\phi_2\, p(\phi_2)\cos(\phi_2)\int_{-\infty}^{+\infty} d\phi_1 p(\phi_1)\int_0^{2\pi}\frac{d\phi_0}{2\pi}\kappa(\phi_2+\phi_1+\phi_0)\kappa(\phi_1+\phi_0). \tag{S29}$$

The auxiliary functions $\kappa(.)$ and their product $\kappa(\phi_2+\phi_1+\phi_0)\kappa(\phi_1+\phi_0)$ are $2\pi$-periodic functions of $\phi_1$. Hence the result of the integration of this product with respect to $\phi_0$ over a period does not depend on $\phi_1$. This simplifies the expression for the correlation function:

$$\langle \Delta k(t_1)\Delta k(t_2)\cos[\phi(t_2)-\phi(t_1)]\rangle = \int_{-\infty}^{+\infty} d\phi_2\, p(\phi_2)\cos(\phi_2)\int_0^{2\pi}\frac{d\phi_0}{2\pi}\kappa(\phi_2+\phi_0)\kappa(\phi_0). \tag{S30}$$

In this equation, the result of integration $\int_0^{2\pi} d\phi_0\kappa(\phi_2+\phi_0)\kappa(\phi_0)/2\pi$, is a $2\pi$-periodic function of $\phi_2$. Let us represent this function by its Fourier series

$$\int_0^{2\pi}\frac{d\phi_0}{2\pi}\kappa(\phi_2+\phi_0)\kappa(\phi_0) = \sum_{n=-\infty}^{+\infty} c_n {\rm e}^{in\phi_2}, \tag{S31}$$

with coefficients

$$c_n = \int_0^{2\pi}\frac{d\phi_2}{2\pi}\,{\rm e}^{-i\phi_2 n}\int_0^{2\pi}\frac{d\phi_0}{2\pi}\kappa(\phi_2+\phi_0)\kappa(\phi_0), \tag{S32}$$

which we evaluate explicitly. To this end, we first perform the integration with respect to $\phi_2$ using Eq. (S19) and the identity ${\rm I}_n(-z) = (-1)^n{\rm I}_n(z)$ valid for integer $n$ and real $z$ [4]. After this we get

$$\int_0^{2\pi}\frac{d\phi_2}{2\pi}\,{\rm e}^{-i\phi_2 n}\kappa(\phi_2+\phi_0) = {\rm e}^{i\phi_0 n}\left[k_+^{(0)} - (-1)^n k_-^{(0)}\right]{\rm I}_n\left(\frac{F\delta r}{2k_{\rm B}T}\right). \tag{S33}$$

Next, we integrate this result multiplied by $\kappa(\phi_0)$ with respect to $\phi_0$ and get the final expression for $c_n$:

$$c_n = \left[k_+^{(0)} - (-1)^n k_-^{(0)}\right]^2 {\rm I}_n^2\left(\frac{F\delta r}{2k_{\rm B}T}\right). \tag{S34}$$

The above procedure can be carried out similarly for the case $t_1 > t_2$, giving us the final result

$$\langle \Delta k(t_1)\Delta k(t_2)\cos[\phi(t_2)-\phi(t_1)]\rangle = \frac{1}{2}\sum_{n=-\infty}^{+\infty}(c_{n-1}+c_{n+1})\,{\rm e}^{-n^2 D_{\rm r}|t_1-t_2|}. \tag{S35}$$

Integration of this formula with respect to $t_1$ and $t_2$ is performed using

$$\int_0^t dt_1 \int_0^t dt_2 \mathrm{e}^{-n^2 D_\mathrm{r}|t_1-t_2|} = \frac{2}{n^4 D_\mathrm{r}^2}\left(\mathrm{e}^{-n^2 D_\mathrm{r} t} - 1\right) + \frac{2t}{n^2 D_\mathrm{r}}, \tag{S36}$$

for $n \neq 0$.

The $n = 0$ term of the series (S35) is time-independent and equal to $(k_+^{(0)} + k_-^{(0)})^2 \, \mathrm{I}_1^2\left(\frac{F\delta r}{2k_\mathrm{B}T}\right)$. In the expression for the variance (S17) it is exactly compensated by the second term on the right-hand side of (S17), see Eq. (S23).

Summing up, for the variance of $\boldsymbol{r}(t)$ we obtain the exact expression

$$\begin{aligned}\langle \boldsymbol{r}^2(t)\rangle - \langle \boldsymbol{r}(t)\rangle^2 = &\left[4D + (\delta r)^2 (k_+^{(0)} + k_-^{(0)})\, \mathrm{I}_0\left(\frac{F\delta r}{2k_\mathrm{B}T}\right)\right] t + \\ &+ (\delta r)^2 \sum_{n\neq 0} [k_+^{(0)} + (-1)^n k_-^{(0)}]^2 \left[\mathrm{I}_{n-1}^2\left(\frac{F\delta r}{2k_\mathrm{B}T}\right) + \mathrm{I}_{n+1}^2\left(\frac{F\delta r}{2k_\mathrm{B}T}\right)\right]\left(\frac{\mathrm{e}^{-n^2 D_\mathrm{r} t} - 1}{n^4 D_\mathrm{r}^2} + \frac{t}{n^2 D_\mathrm{r}}\right).\end{aligned} \tag{S37}$$

In agreement with discussion in the main text, this results can be expressed in terms of mean active velocity and active diffusivity of an un-forced active dynamics: Furthermore, identifying

$$v_\mathrm{a}^{(0)} = \delta r (k_+^{(0)} - k_-^{(0)}), \tag{S38}$$

$$D_\mathrm{a}^{(0)} = \frac{(\delta r)^2}{2}(k_+^{(0)} + k_-^{(0)}). \tag{S39}$$

We obtain

$$\begin{aligned}\langle \boldsymbol{r}^2(t)\rangle - \langle \boldsymbol{r}(t)\rangle^2 = &\left[4D + 2D_\mathrm{a}^{(0)}\, \mathrm{I}_0\left(\frac{F\delta r}{2k_\mathrm{B}T}\right)\right] t + \\ &+ 4\left(\frac{D_\mathrm{a}^{(0)}}{\delta r}\right)^2 \sum_{n\ \mathrm{even}, n\neq 0} \left[\mathrm{I}_{n-1}^2\left(\frac{F\delta r}{2k_\mathrm{B}T}\right) + \mathrm{I}_{n+1}^2\left(\frac{F\delta r}{2k_\mathrm{B}T}\right)\right]\left(\frac{\mathrm{e}^{-n^2 D_\mathrm{r} t} - 1}{n^4 D_\mathrm{r}^2} + \frac{t}{n^2 D_\mathrm{r}}\right) + \\ &+ (v_\mathrm{a}^{(0)})^2 \sum_{n\ \mathrm{odd}} \left[\mathrm{I}_{n-1}^2\left(\frac{F\delta r}{2k_\mathrm{B}T}\right) + \mathrm{I}_{n+1}^2\left(\frac{F\delta r}{2k_\mathrm{B}T}\right)\right]\left(\frac{\mathrm{e}^{-n^2 D_\mathrm{r} t} - 1}{n^4 D_\mathrm{r}^2} + \frac{t}{n^2 D_\mathrm{r}}\right).\end{aligned} \tag{S40}$$

### C. Weak-force approximation

In the weak-force (pN and less) limit, $F\delta r/2k_\mathrm{B}T < 1$, we expand the Bessel functions in above equations. Namely, we use [4] $\mathrm{I}_0(z) = 1 + z^2/4 + O(x^4)$, and $\mathrm{I}_1(z) = \mathrm{I}_{-1}(z) = z/2 + O(x^3)$. Higher order Bessel functions yield higher powers of the ratio $(F\delta r/2k_\mathrm{B}T)$ and can be neglected.

As for mean values, we get

$$\langle x(t)\rangle = \left[\mu + \frac{(\delta r)^2}{4k_\mathrm{B}T}(k_+^{(0)} + k_-^{(0)})\right] Ft. \tag{S41}$$

The variance (S37) is given by

$$\begin{aligned}\langle \boldsymbol{r}^2(t)\rangle - \langle \boldsymbol{r}(t)\rangle^2 = &\left\{4D + (\delta r)^2 (k_+^{(0)} + k_-^{(0)})\left[1 + \frac{1}{16}\left(\frac{F\delta r}{k_\mathrm{B}T}\right)^2\right]\right\} t + \\ &+ (\delta r)^2 (k_+^{(0)} - k_-^{(0)})^2 \left[2 + \frac{1}{4}\left(\frac{F\delta r}{k_\mathrm{B}T}\right)^2\right]\left(\frac{\mathrm{e}^{-D_\mathrm{r} t} - 1}{D_\mathrm{r}^2} + \frac{t}{D_\mathrm{r}}\right) \\ &+ \frac{(\delta r)^2}{32}(k_+^{(0)} + k_-^{(0)})^2 \left(\frac{F\delta r}{k_\mathrm{B}T}\right)^2 \left(\frac{\mathrm{e}^{-4D_\mathrm{r} t} - 1}{4D_\mathrm{r}^2} + \frac{t}{D_\mathrm{r}}\right).\end{aligned} \tag{S42}$$

As it is used in the main text, we express these quantities using Eqs. (S38) and (S39) as follows

$$\langle x(t)\rangle = \left(\mu + \frac{1}{2}\frac{D_\mathrm{a}^{(0)}}{k_\mathrm{B}T}\right) Ft, \tag{S43}$$

and

$$\langle \boldsymbol{r}^2(t)\rangle - \langle \boldsymbol{r}(t)\rangle^2 = \left\{4D + 2D_{\rm a}^{(0)}\left[1+\left(\frac{F\delta r}{4k_{\rm B}T}\right)^2\right]\right\} t + \\ + 2\frac{(v_{\rm a}^{(0)})^2}{D_{\rm r}}\left[1+\frac{1}{8}\left(\frac{F\delta r}{k_{\rm B}T}\right)^2\right]\left(\frac{{\rm e}^{-D_{\rm r}t}-1}{D_{\rm r}}+t\right) + \frac{1}{8D_{\rm r}}\left(\frac{D_{\rm a}^{(0)}F}{k_{\rm B}T}\right)^2\left(\frac{{\rm e}^{-4D_{\rm r}t}-1}{4D_{\rm r}}+t\right). \tag{S44}$$

### D. Zero-force case: Comparison with experiments

With zero external forcing, we have $\langle x(t)\rangle = \langle y(t)\rangle = 0$, and

$$\langle \boldsymbol{r}^2(t)\rangle - \langle \boldsymbol{r}(t)\rangle^2 = 4\left[D + \frac{(\delta r)^2}{4}(k_+^{(0)}+k_-^{(0)})\right] t + 2\frac{(\delta r)^2}{D_{\rm r}^2}(k_+^{(0)}-k_-^{(0)})^2\left({\rm e}^{-D_{\rm r}t}-1+D_{\rm r}t\right), \tag{S45}$$

hence we have

$$\mathcal{D}^{(0)} = \lim_{t\to\infty}\frac{\langle \boldsymbol{r}^2(t)\rangle - \langle \boldsymbol{r}(t)\rangle^2}{4t} = D + \frac{(\delta r)^2}{4}(k_+^{(0)}+k_-^{(0)}) + \frac{(\delta r)^2}{2D_{\rm r}}(k_+^{(0)}-k_-^{(0)})^2. \tag{S46}$$

Using definitions (S38) and (S39), we can write these result as

$$\langle \boldsymbol{r}^2(t)\rangle - \langle \boldsymbol{r}(t)\rangle^2 = \left(4D + 2D_{\rm a}^{(0)}\right)t + 2\left(\frac{v_{\rm a}^{(0)}}{D_{\rm r}}\right)^2\left({\rm e}^{-D_{\rm r}t}-1+D_{\rm r}t\right), \tag{S47}$$

and

$$\mathcal{D}^{(0)} = D + \frac{D_{\rm a}^{(0)}}{2} + \frac{(v_{\rm a}^{(0)})^2}{2D_{\rm r}}. \tag{S48}$$

Furthermore, one can assume a specific form of rates $k_\pm^{(0)}$, e.g.,

$$k_\pm^{(0)} = \mu_{\rm c}\frac{k_{\rm B}T}{(\delta r)^2}\exp\left(\pm\frac{\Delta G_{\rm r}}{2k_{\rm B}T}\right), \tag{S49}$$

then we have

$$k_+^{(0)} + k_-^{(0)} = 2\frac{\mu_{\rm c}k_{\rm B}T}{(\delta r)^2}\cosh\left(\frac{\Delta G_{\rm r}}{2k_{\rm B}T}\right), \tag{S50}$$

$$k_+^{(0)} - k_-^{(0)} = 2\frac{\mu_{\rm c}k_{\rm B}T}{(\delta r)^2}\sinh\left(\frac{\Delta G_{\rm r}}{2k_{\rm B}T}\right), \tag{S51}$$

and for the diffusivity we obtain

$$\mathcal{D}^{(0)} = k_{\rm B}T\left[\mu + \frac{\mu_{\rm c}}{2}\cosh\left(\frac{\Delta G_{\rm r}}{2k_{\rm B}T}\right)\right] + \frac{2}{D_{\rm r}}\left(\frac{\mu_{\rm c}k_{\rm B}T}{\delta r}\right)^2\sinh^2\left(\frac{\Delta G_{\rm r}}{2k_{\rm B}T}\right). \tag{S52}$$

## II. MACROSCOPIC LIMIT FOR THE THERMODYNAMICALLY CONSISTENT PROPULSION

By the macroscopic limit we understand transition from time- and length-scales where individual active jumps can be resolved to the ones where the active velocity can be represented by a continuous process with a non-fluctuating deterministic part and a stochastic part described by white noise.

At microscopic scales, every chemical reaction induces a shift of the active particle along its orientation $\boldsymbol{n}$ by $\delta r$. Microscopic reversibility guarantees that there exists also a backward reaction associated with a shift by $\delta r$ along the opposite direction $-\boldsymbol{n}$. Transition rates of the forward ($k_+$) and the backward ($k_-$) processes are detailed balanced locally

$$\frac{k_+(\boldsymbol{r}\to\boldsymbol{r}+\boldsymbol{n}\delta r)}{k_-(\boldsymbol{r}+\boldsymbol{n}\delta r\to\boldsymbol{r})} = \exp[\Delta S(\boldsymbol{r}\to\boldsymbol{r}+\boldsymbol{n}\delta r)], \tag{S53}$$

where $\Delta S(\boldsymbol{r} \to \boldsymbol{r} + \boldsymbol{n}\delta r)$ denotes the entropy produced in the universe after the forward process. It consists of two terms

$$\Delta S(\boldsymbol{r} \to \boldsymbol{r} + \boldsymbol{n}\delta r) = \frac{\Delta G_{\mathrm{r}} - \delta W(\boldsymbol{r} \to \boldsymbol{r} + \boldsymbol{n}\delta r)}{k_{\mathrm{B}}T}, \tag{S54}$$

the first is an $\boldsymbol{r}$-independent free energy of the forward reaction, which we parametrize by the ratio

$$\Delta G_{\mathrm{r}} = \frac{u}{\mu_{\mathrm{c}}}\delta r, \tag{S55}$$

where the free energy needed to move a particle by $\delta r$ is given in terms of a velocity $u$ and mobility $\mu_{\mathrm{c}}$.

The second term on the right-hand side of (S54) stands for the work done against external mechanical force $\boldsymbol{F}(\boldsymbol{r})$ arising from the potential $V(\boldsymbol{r})$, i.e., $\boldsymbol{F}(\boldsymbol{r}) = -\nabla V(\boldsymbol{r})$. Namely, we have

$$\delta W(\boldsymbol{r} \to \boldsymbol{r} + \boldsymbol{n}\delta r) = V(\boldsymbol{r} + \boldsymbol{n}\delta r) - V(\boldsymbol{r}). \tag{S56}$$

Considering only the terms in the master equation (S3) describing the active propulsion (i.e., disregarding the passive diffusion), we have

$$\begin{aligned}\partial_t P(\boldsymbol{r}, t) = {} & k_+(\boldsymbol{r} - \boldsymbol{n}\delta r \to \boldsymbol{r})P(\boldsymbol{r} - \boldsymbol{n}\delta r, t) + k_-(\boldsymbol{r} + \boldsymbol{n}\delta r \to \boldsymbol{r})P(\boldsymbol{r} + \boldsymbol{n}\delta r, t) \\ & - \left[k_+(\boldsymbol{r} \to \boldsymbol{r} + \boldsymbol{n}\delta r) + k_-(\boldsymbol{r} \to \boldsymbol{r} - \boldsymbol{n}\delta r)\right] P(\boldsymbol{r}, t).\end{aligned} \tag{S57}$$

A specific choice of rates $k_\pm$ (Glauber, exponential, etc.) does not alter the coarsegrained description on macroscopic length and time scales. Let us choose rates for the processes $\boldsymbol{r} \rightleftharpoons \boldsymbol{r} + \boldsymbol{n}\delta r$, in the frequently used exponential form

$$k_\pm(\boldsymbol{r} \to \boldsymbol{r} + \boldsymbol{n}\delta r) = \frac{D_{\mathrm{c}}}{(\delta r)^2} \exp\left[\pm\frac{1}{2}\Delta S(\boldsymbol{r} \to \boldsymbol{r} + \boldsymbol{n}\delta r)\right], \tag{S58}$$

where $D_{\mathrm{c}}$ satisfies the fluctuation-dissipation theorem

$$D_{\mathrm{c}} = \mu_{\mathrm{c}} k_{\mathrm{B}} T. \tag{S59}$$

The rate constants for process $\boldsymbol{r} - \boldsymbol{n}\delta r \rightleftharpoons \boldsymbol{r}$, $k_\pm(\boldsymbol{r} - \boldsymbol{n}\delta r \to \boldsymbol{r})$, are given by analogous expressions.

In the limit $\delta r \to 0$, we expand the rate constants as follows

$$k_+(\boldsymbol{r} \to \boldsymbol{r} + \boldsymbol{n}\delta r) \approx \frac{D_{\mathrm{c}}}{(\delta r)^2}\left\{1 + \frac{\delta r}{2k_{\mathrm{B}}T}\left(\frac{u}{\mu_{\mathrm{c}}} - \partial_n V(\boldsymbol{r})\right) + \frac{(\delta r)^2}{8(k_{\mathrm{B}}T)^2}\left[\left(\frac{u}{\mu_{\mathrm{c}}} - \partial_n V(\boldsymbol{r})\right)^2 - 2k_{\mathrm{B}}T\partial_n^2 V(\boldsymbol{r})\right]\right\}, \tag{S60}$$

$$k_-(\boldsymbol{r} + \boldsymbol{n}\delta r \to \boldsymbol{r}) \approx \frac{D_{\mathrm{c}}}{(\delta r)^2}\left\{1 - \frac{\delta r}{2k_{\mathrm{B}}T}\left(\frac{u}{\mu_{\mathrm{c}}} - \partial_n V(\boldsymbol{r})\right) + \frac{(\delta r)^2}{8(k_{\mathrm{B}}T)^2}\left[\left(\frac{u}{\mu_{\mathrm{c}}} - \partial_n V(\boldsymbol{r})\right)^2 + 2k_{\mathrm{B}}T\partial_n^2 V(\boldsymbol{r})\right]\right\}, \tag{S61}$$

$$k_+(\boldsymbol{r} - \boldsymbol{n}\delta r \to \boldsymbol{r}) \approx \frac{D_{\mathrm{c}}}{(\delta r)^2}\left\{1 + \frac{\delta r}{2k_{\mathrm{B}}T}\left(\frac{u}{\mu_{\mathrm{c}}} - \partial_n V(\boldsymbol{r})\right) + \frac{(\delta r)^2}{8(k_{\mathrm{B}}T)^2}\left[\left(\frac{u}{\mu_{\mathrm{c}}} - \partial_n V(\boldsymbol{r})\right)^2 + 2k_{\mathrm{B}}T\partial_n^2 V(\boldsymbol{r})\right]\right\}, \tag{S62}$$

$$k_-(\boldsymbol{r} \to \boldsymbol{r} - \boldsymbol{n}\delta r) \approx \frac{D_{\mathrm{c}}}{(\delta r)^2}\left\{1 - \frac{\delta r}{2k_{\mathrm{B}}T}\left(\frac{u}{\mu_{\mathrm{c}}} - \partial_n V(\boldsymbol{r})\right) + \frac{(\delta r)^2}{8(k_{\mathrm{B}}T)^2}\left[\left(\frac{u}{\mu_{\mathrm{c}}} - \partial_n V(\boldsymbol{r})\right)^2 - 2k_{\mathrm{B}}T\partial_n^2 V(\boldsymbol{r})\right]\right\}, \tag{S63}$$

where we have introduced the directional derivative along the vector $\boldsymbol{n}$,

$$\partial_n = \boldsymbol{n} \cdot \nabla = \cos\phi\,\partial_x + \sin\phi\,\partial_y, \tag{S64}$$

since we have $(\boldsymbol{r} + \boldsymbol{n}\delta r) = (x + \delta r\cos\phi, y + \delta r\sin\phi)$,

Introducing expansions (S60)-(S63) into the master equation (S57), where we expand terms $P(\boldsymbol{r} \pm \boldsymbol{n}\delta r, t)$ along similar lines, gives us the diffusive dynamics along the direction $\boldsymbol{n}$. The dynamics is governed by the Fokker-Planck equation

$$\partial_t P = \mathcal{L}_{\mathrm{a}} P, \tag{S65}$$

with the Fokker-Planck operator

$$\mathcal{L}_{\mathrm{a}} = -u\partial_n + \mu_{\mathrm{c}}\partial_n\left[k_{\mathrm{B}}T\partial_n - F_n(\boldsymbol{r}, \phi)\right], \tag{S66}$$

which is expressed using the force projection on the particle orientation:

$$F_n(\boldsymbol{r},\phi) = \boldsymbol{n}\cdot\boldsymbol{F}(\boldsymbol{r}) = -\partial_n V(\boldsymbol{r}). \tag{S67}$$

Let us further introduce the standard Fokker-Planck operator for a passive Brownian motion

$$\mathcal{L} = \mu\nabla\cdot\left[k_{\mathrm{B}}T\,\nabla - \boldsymbol{F}(\boldsymbol{r})\right], \tag{S68}$$

and the one for the rotational diffusion containing derivatives with respect to the angle $\phi$,

$$\mathcal{L}_{\mathrm{r}} = D_{\mathrm{r}}\partial^2_{\phi\phi}. \tag{S69}$$

Then the Fokker-Planck equation for the joint PDF $p(\boldsymbol{r},\phi,t)$ of the particle position $\boldsymbol{r}$ and angle $\phi$ at time $t$ is given by

$$\partial_t p(\boldsymbol{r},\phi,t) = \left(\mathcal{L}+\mathcal{L}_{\mathrm{a}}+\mathcal{L}_{\mathrm{r}}\right)p(\boldsymbol{r},\phi,t). \tag{S70}$$

Therefore, dynamics of $\boldsymbol{r}(t)$ is governed by the Langevin equations corresponding to the Fokker-Planck equation (S70):

$$\frac{d\boldsymbol{r}}{dt} = \left[u + \mu_{\mathrm{c}}F_n(\boldsymbol{r},t) + \sqrt{2D_{\mathrm{c}}}\,\xi_n(t)\right]\boldsymbol{n}(t) + \mu\boldsymbol{F}(\boldsymbol{r}) + \sqrt{2D}\,\boldsymbol{\xi}(t), \tag{S71}$$

where the white noise $\xi_n(t)$ arising from fluctuations in a number of chemical reactions satisfies $\langle\xi_n(t)\rangle = 0$ and $\langle\xi_n(t)\xi_n(t')\rangle = \delta(t-t')$. It is independent of the white noise of the passive Brownian motion $\boldsymbol{\xi}(t) = (\xi_x(t),\xi_y(t))$ with $\langle\xi_x(t)\rangle = \langle\xi_y(t)\rangle = 0$ and $\langle\xi_i(t)\xi_j(t')\rangle = \delta_{ij}\delta(t-t')$, $i,j = x,y$. The Langevin equation for the particle position (S71) is further supplemented by the Langevin equation (S1) giving evolution of particle orientation.

## III. POSITION STATISTICS IN MACROSCOPIC LIMIT

In this section, moments of the particle position are studied based on the Langevin equation (S71). First, in the auxiliary subsection III A necessary properties of the process $\phi(t)$ are summarized, which are ten used in Subsec. III B to calculate averages discussed in the main text.

### A. Correlation functions in rotational diffusion

To evaluate the diffusion coefficient of a particle, we shall need the following expressions for averages and correlation functions of $\cos\phi(t)$ and $\sin\phi(t)$. Their evaluation is based on the fact that $\phi(t)$ is a Gaussian process, cf. Eq. (S2). Namely, in the calculations, one can first express all trigonometric functions as sums of complex exponentials and then perform averages of theses exponentials, where the exponents are Gaussian random variables. Thanks to properties of the Gaussian process any such calculation reduces to computations of two-time correlation functions via Wick's probability theorem.

For the mean values of $\sin\phi(t)$ and $\cos\phi(t)$ and for a fixed $\phi_0$ we get

$$\langle\sin\phi(t)\rangle = \langle\sin\phi_0\rangle \mathrm{e}^{-D_{\mathrm{r}}t}, \tag{S72}$$

$$\langle\cos\phi(t)\rangle = \langle\cos\phi_0\rangle \mathrm{e}^{-D_{\mathrm{r}}t}, \tag{S73}$$

respectively. Averages $\langle\sin\phi_0\rangle$ and $\langle\cos\phi_0\rangle$ over $\phi_0\in[0,2\pi)$ are equal to zero hence $\langle\sin\phi(t)\rangle$ and $\langle\cos\phi(t)\rangle$ also vanish for all $t$ meaning there is no preferred orientation, i.e., $\langle\boldsymbol{n}(t)\rangle = \boldsymbol{0}$.

The following two-time correlation functions shall appear in course of calculations:

$$\langle\cos\phi(t_1)\cos\phi(t_2)\rangle = \frac{1}{2}\mathrm{e}^{-D_{\mathrm{r}}|t_1-t_2|}, \tag{S74}$$

$$\langle\sin\phi(t_1)\sin\phi(t_2)\rangle = \frac{1}{2}\mathrm{e}^{-D_{\mathrm{r}}|t_1-t_2|}, \tag{S75}$$

$$\langle\sin\phi(t_1)\cos\phi(t_2)\rangle = 0, \tag{S76}$$

$$\langle\cos^2\phi(t_1)\cos\phi(t_2)\rangle = 0, \tag{S77}$$

$$\langle\sin^2\phi(t_1)\cos\phi(t_2)\rangle = 0, \tag{S78}$$

$$\langle\cos^2\phi(t_1)\cos^2\phi(t_2)\rangle = \frac{1}{4} + \frac{1}{8}\mathrm{e}^{-4D_{\mathrm{r}}|t_1-t_2|}. \tag{S79}$$

Finally, we shall also use the following result for the four-time correlation function

$$\langle \sin\phi(t_1)\cos\phi(t_1)\sin\phi(t_2)\cos\phi(t_2)\rangle = \frac{1}{4}\langle \sin(2\phi(t_1))\sin(2\phi(t_2))\rangle = \frac{1}{8}\mathrm{e}^{-4D_\mathrm{r}|t_1-t_2|}. \tag{S80}$$

### B. Moments of the particle position

Projection of the external constant force $\boldsymbol{F} = (F, 0)$ onto a particle orientation $\boldsymbol{n}$ is given by the time-dependent expression $F_n(t) = \boldsymbol{n}(t)\cdot\boldsymbol{F} = F\cos\phi(t)$, cf. Eq. (S67). The projection appears in both Langevin equations governing dynamics of coordinates $x(t)$ and $y(t)$. In the equation for $x(t)$ $[y(t)]$, it is multiplied by $\mu_\mathrm{c}\cos\phi(t)$ $[\mu_\mathrm{c}\sin\phi(t)]$. Integrating these equations subject to given initial conditions at $t = 0$, we obtain

$$x(t) = x(0) + \int_0^t \left[\mu F + \mu_\mathrm{c} F\cos^2\phi(t') + u\cos\phi(t')\right] dt' + \int_0^t \left[\sqrt{2D}\,\xi_x(t') + \sqrt{2D_\mathrm{c}}\,\xi_n(t')\cos\phi(t')\right] dt', \tag{S81}$$

$$y(t) = y(0) + \int_0^t \left[\mu_\mathrm{c} F\cos\phi(t')\sin\phi(t') + u\sin\phi(t')\right] dt' + \int_0^t \left[\sqrt{2D}\,\xi_y(t') + \sqrt{2D_\mathrm{c}}\,\xi_n(t')\sin\phi(t')\right] dt'. \tag{S82}$$

Assuming the initial particle position to be at the origin, $x(0) = y(0) = 0$, and using Eqs. (S72), (S73), (S74), and (S76), we get the description of average particle motion:

$$\langle x(t)\rangle = \left(\mu + \frac{\mu_\mathrm{c}}{2}\right) Ft, \tag{S83}$$

$$\langle y(t)\rangle = 0. \tag{S84}$$

Calculations of second moments is somewhat more cumbersome, yet it runs along similar lines: averaging $x^2(t)$ and $y^2(t)$ is performed with the aid of Eqs. (S72)-(S79). Setting again $x(0) = y(0) = 0$, the final results of this calculation assumes the form

$$\langle x^2(t)\rangle = \left(\mu + \frac{\mu_\mathrm{c}}{2}\right)^2 (Ft)^2 + 2\left(D + \frac{D_\mathrm{c}}{2}\right)t + \left(\frac{u}{D_\mathrm{r}}\right)^2\left(D_\mathrm{r}t + \mathrm{e}^{-D_\mathrm{r}t} - 1\right) + \left(\frac{\mu_\mathrm{c}F}{8D_\mathrm{r}}\right)^2\left(4D_\mathrm{r}t + \mathrm{e}^{-4D_\mathrm{r}t} - 1\right), \tag{S85}$$

$$\langle y^2(t)\rangle = 2\left(D + \frac{D_\mathrm{c}}{2}\right)t + \left(\frac{u}{D_\mathrm{r}}\right)^2\left(D_\mathrm{r}t + \mathrm{e}^{-D_\mathrm{r}t} - 1\right) + \left(\frac{\mu_\mathrm{c}F}{8D_\mathrm{r}}\right)^2\left(4D_\mathrm{r}t + \mathrm{e}^{-4D_\mathrm{r}t} - 1\right). \tag{S86}$$

Along $x$ and $y$ directions, diffusive spreading of the probability density function for the particle position is described by the second central moments $\langle x^2(t)\rangle - \langle x(t)\rangle^2$ and $\langle y^2(t)\rangle - \langle y(t)\rangle^2$. Comparing above equations, we observe that $\langle x^2(t)\rangle - \langle x(t)\rangle^2 = \langle y^2(t)\rangle - \langle y(t)\rangle^2$ holds. Hence for the squared deviation of $\boldsymbol{r}$ from its mean we have

$$\langle \boldsymbol{r}^2(t)\rangle - \langle \boldsymbol{r}(t)\rangle^2 = 2[\langle x^2(t)\rangle - \langle x(t)\rangle^2] = 2[\langle y^2(t)\rangle - \langle y(t)\rangle^2] = 2\langle y^2(t)\rangle. \tag{S87}$$

which gives us

$$\langle \boldsymbol{r}^2(t)\rangle - \langle \boldsymbol{r}(t)\rangle^2 = 4\left(D + \frac{D_\mathrm{c}}{2}\right)t + 2\left(\frac{u}{D_\mathrm{r}}\right)^2\left(D_\mathrm{r}t + \mathrm{e}^{-D_\mathrm{r}t} - 1\right) + 2\left(\frac{\mu_\mathrm{c}F}{8D_\mathrm{r}}\right)^2\left(4D_\mathrm{r}t + \mathrm{e}^{-4D_\mathrm{r}t} - 1\right). \tag{S88}$$

In the short-time limit $D_\mathrm{r}t \ll 1$, the exponential functions in Eq. (S88) can be expanded into power series yielding

$$\langle \boldsymbol{r}^2(t)\rangle - \langle \boldsymbol{r}(t)\rangle^2 \approx 4\left(D + \frac{D_\mathrm{c}}{2}\right)t, \qquad D_\mathrm{r}t \ll 1. \tag{S89}$$

On the other hand, in the long-time limit the exponentials in Eq. (S88) vanish and we end up with the linear time dependence

$$\langle \boldsymbol{r}^2(t)\rangle - \langle \boldsymbol{r}(t)\rangle^2 \approx 4\left[D + \frac{D_\mathrm{c}}{2} + \frac{u^2}{2D_\mathrm{r}} + \frac{(\mu_\mathrm{c}F)^2}{32D_\mathrm{r}}\right]t - 2\left[\left(\frac{u}{D_\mathrm{r}}\right)^2 + \left(\frac{\mu_\mathrm{c}F}{8D_\mathrm{r}}\right)^2\right], \qquad D_\mathrm{r}t \gg 1. \tag{S90}$$


[1] P. Pietzonka and U. Seifert, Entropy production of active particles and for particles in active baths, J. Phys. A **51**, 01LT01 (2018).

[2] T. Speck, Active Brownian particles driven by constant affinity, EPL **123**, 20007 (2018).

[3] T. Speck, Thermodynamic approach to the self-diffusiophoresis of colloidal Janus particles, Phys. Rev. E **99**, 060602 (2019).

[4] M. Abramowitz and I. A. Stegun, *Handbook of Mathematical Functions with Formulas, Graphs, and Mathematical Tables*, ninth dover printing, tenth gpo printing ed. (New York, 1964).
